# Supplementary material for: Size Growth on Short Timescales of Star-Forming Galaxies: Insights from Size Variation with Rest-Frame Wavelength with JADES
Source: arXiv:2411.07458 source file (2024-11-12)
Supplement: Supplementary file 1 [file Appendix.tex]

The samples of galaxies .... 

\begin{figure}
    \centering
    \includegraphics[scale=0.35]{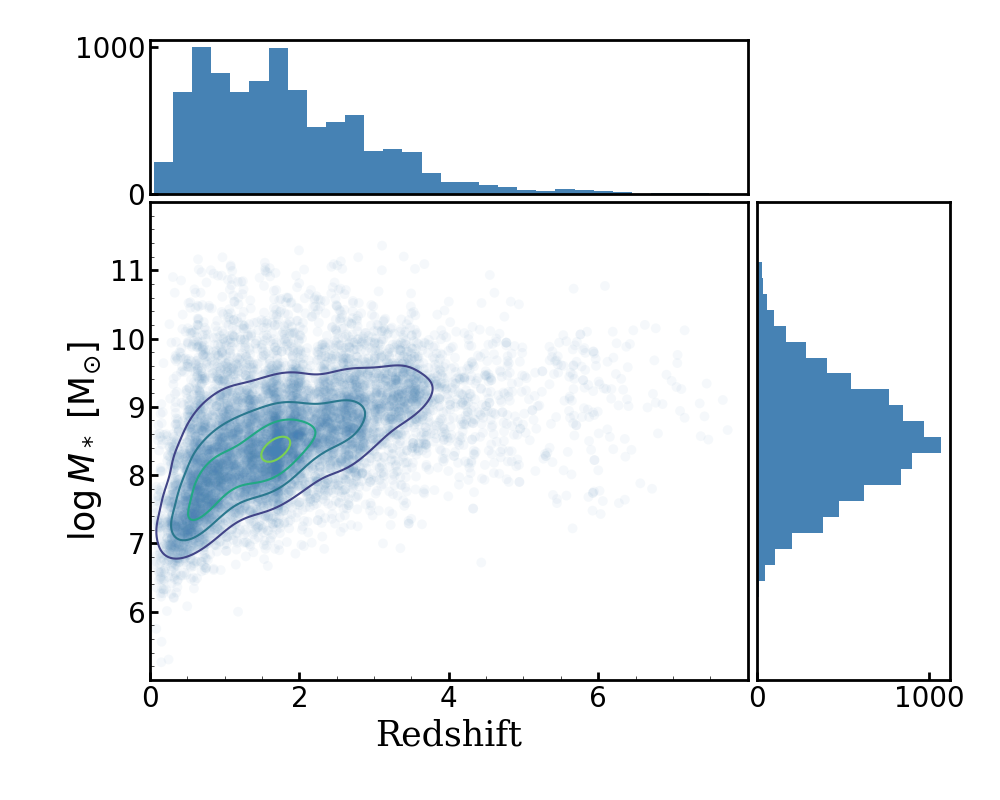}
    \caption{Distribution of sample matched in both JADES catalog \citep{2023arXiv231012340E} and CANDELS catalog \citep{2015ApJ...801...97S}. Blue horizontal line indicates our cut of $M_*$, where $M_*=8$.}
    \label{Fig.1}
\end{figure}

The size variation with wavelength for individual galaxies ...
